# Supplementary material for: Radiation damage and phase stability of Al$_x$CrCuFeNi$_y$ alloys using a machine-learned interatomic potential
Source: arXiv:2503.07344 source file (2025-08-27)
Supplement: Supplementary file 1 [file supplemental.pdf]

# Supplemental material for: Radiation damage and phase stability of $Al_xCrCuFeNi_y$ alloys using a machine-learned interatomic potential

A. Fellman,[1,*] J. Byggmästar,[1] F. Granberg,[1] F. Djurabekova,[1] and K. Nordlund[1]

[1] *Department of Physics, P.O. Box 43, FI-00014 University of Helsinki, Finland*

(Dated: March 10, 2025)

## S1. HYPERPARAMETERS OF THE GAP FITTING

TABLE S1: Hyperparameters used for the different descriptors: cutoff radius $r_{\mathrm{cut}}$, width of the cutoff region $r_{\Delta\mathrm{cut}}$, energy prefactor $\delta$, and the number of sparse descriptor environments from the training structures $M$.

| Descriptor | $r_{\mathrm{cut}}$ (Å) | $r_{\Delta\mathrm{cut}}$ (Å) | $\delta$ | $M$ |
|---|---|---|---|---|
| 2b | 5.2 | 1.0 | 10 | 20 |
| EAM | 5.2 | 1.0 | 1.0 | 30 |
| 3b | 4.7 | 0.6 | 1.0 | 500 |

## S2. RELATIVE FORMATION ENERGY OF UNORDERED BINARIES

In addition to mixing energies the formation energies of the binaries was calculated based on the following equation:

$$E_{\mathrm{f}} = (E_{\mathrm{tot}} - N_A E_A - N_B E_B)/N_{\mathrm{tot}} \tag{1}$$

Where $E_A$ and $E_B$ are the energies per atom for the single element compositions in the lowest energy crystal structure. Fig. S1 shows the formation energies of the constituent binary alloys, where the BCC formation energy has been subtracted from the FCC formation energy. Here the same data is used as in the mixing energies as in the manuscript. The figure gives insight into the energetically favored crystal structures as a function of concentration with the exception of possible ordered structures which might be more stable. In the figure negative formation energies are to be interpreted as FCC being energetically more favorable and positive mean BCC is favored.

* Corresponding author; aslak.fellman@helsinki.fi

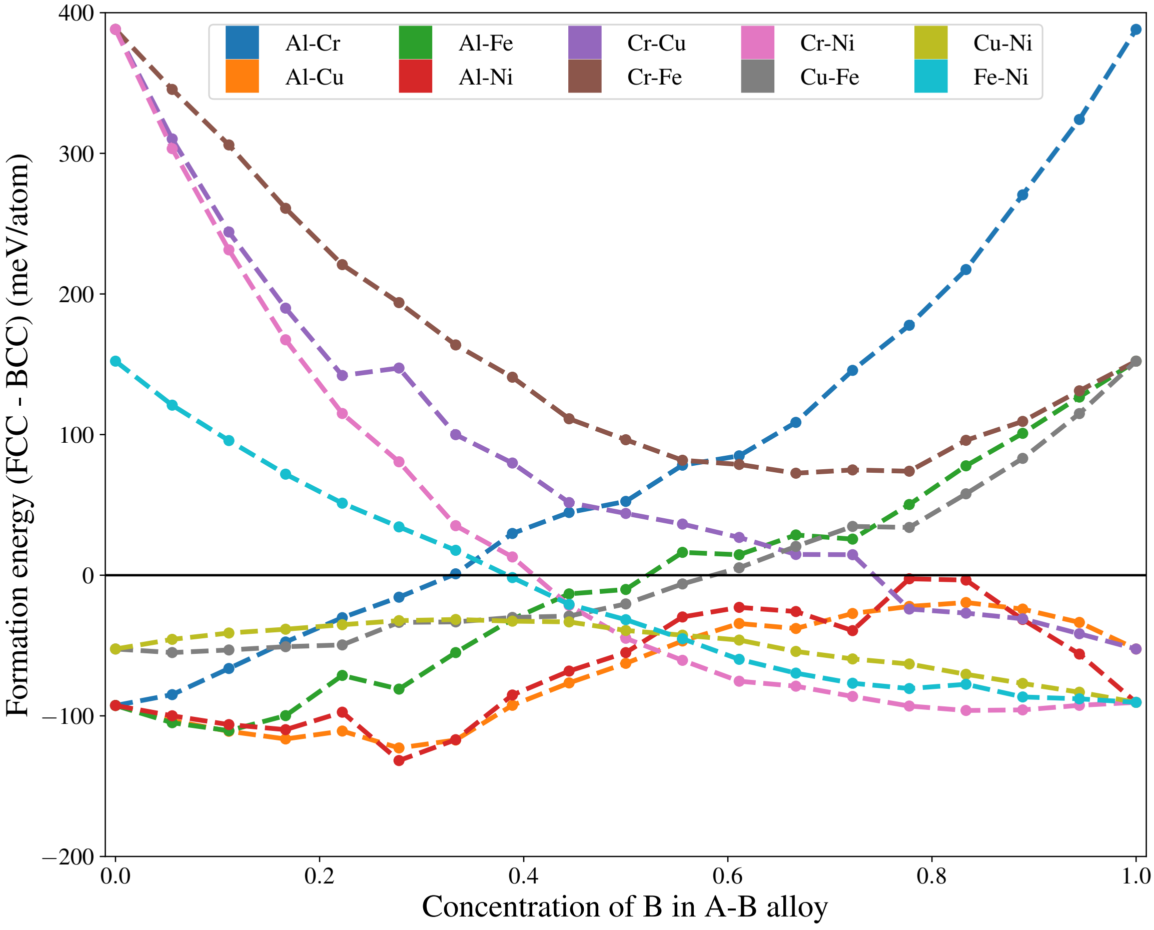


FIG. S1: Formation energy (BCC subtracted from FCC) of constituent binary alloys with varying compositions. Negative values mean FCC energetically favored and positive values mean BCC favored.

## S3. VACANCY FORMATION ENERGY DISTRIBUTIONS

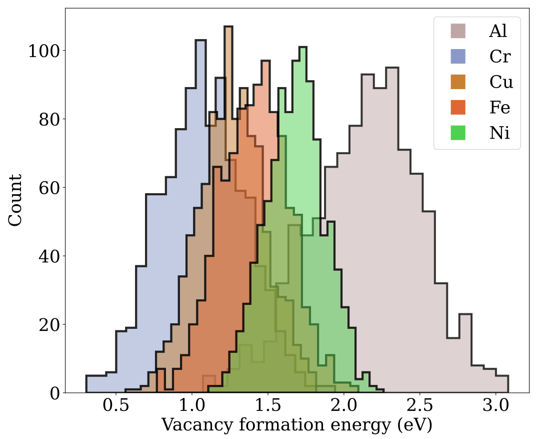


(a) $Al_{0.5}CrCuFeNi$

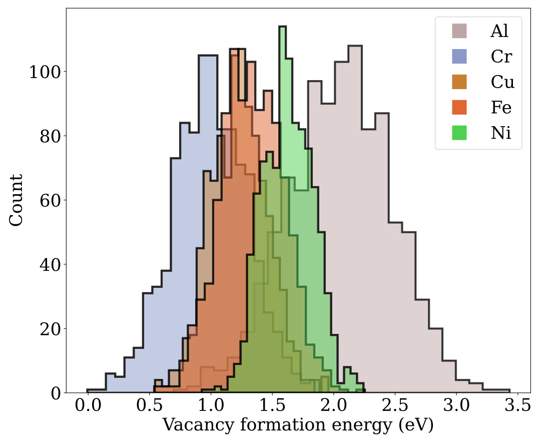


(b) $AlCrCuFeNi_2$

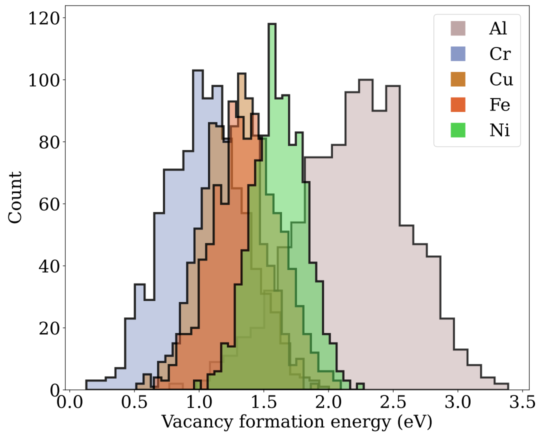


(c) $AlCrCuFeNi_3$

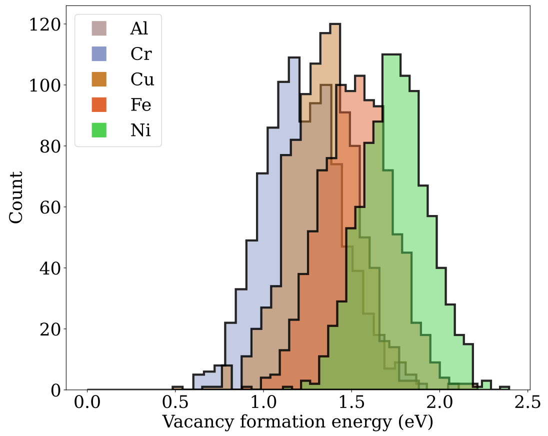


(d) CrCuFeNi

FIG. S2: Distribution of vacancy formation energies of different chemical types in different compositions from 1000 random configurations. Number of bins in the histogram was 25.

## S4. SHORT-RANGE ORDERING

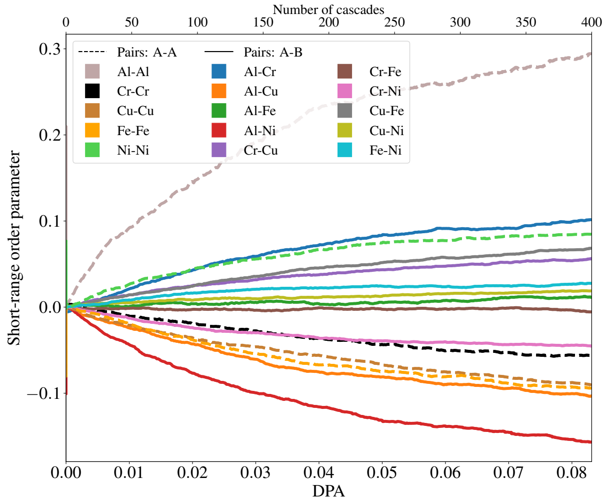


(a) $Al_{0.5}CrCuFeNi$

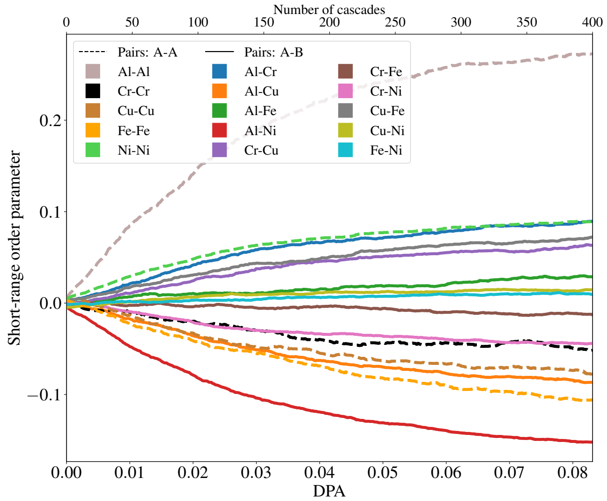


(b) $AlCrCuFeNi_2$

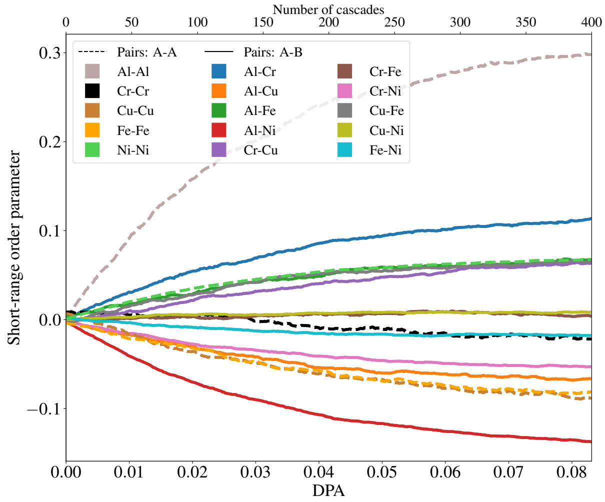


(c) $AlCrCuFeNi_3$

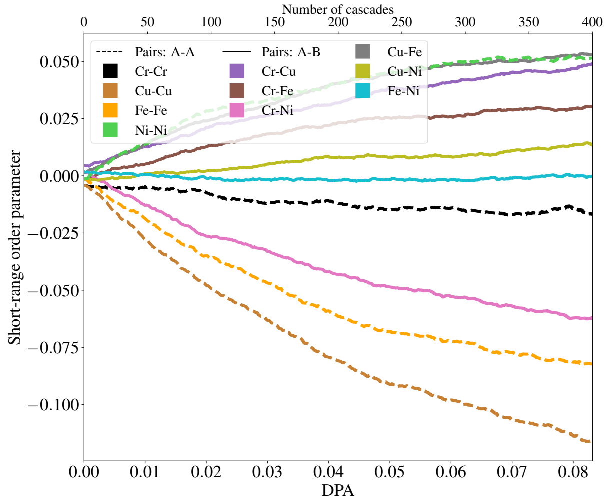


(d) CrCuFeNi

FIG. S3: Short-range order parameters (first shell) for all element pairs in different compositions during the overlapping cascades. The dashed lines represent all pair with the same chemical type and the others are between pairs of different chemical types.

TABLE S2: Short-range order parameters for all element pairs in the final structures of the Monte Carlo MD simulations for the smaller boxes initially in FCC. AlCrCuFeNi uses BCC lattice constant to define first shell as final structure is BCC.

| composition | Al-Al | Al-Cr | Al-Cu | Al-Fe | Al-Ni | Cr-Cr | Cr-Cu | Cr-Fe | Cr-Ni | Cu-Cu | Cu-Fe | Cu-Ni | Fe-Fe | Fe-Ni | Ni-Ni |
|---|---|---|---|---|---|---|---|---|---|---|---|---|---|---|---|
| AlCrCuFeNi | 0.965 | 0.794 | -0.029 | 0.084 | -1.814 | -2.408 | 0.759 | -0.005 | 0.857 | -0.969 | 0.639 | -0.417 | -1.433 | 0.696 | 0.58 |
| $AlCrCuFeNi_2$ | 0.613 | 0.569 | -0.42 | 0.468 | -0.62 | -0.65 | 0.923 | -1.53 | 0.343 | -1.04 | 0.93 | -0.19 | -0.80 | 0.471 | -0.001 |
| $AlCrCuFeNi_3$ | 1.000 | 0.894 | -0.964 | 0.843 | -0.588 | -0.447 | 0.887 | -1.771 | 0.143 | -0.399 | 0.976 | -0.168 | -1.529 | 0.495 | 0.039 |
| $Al_{0.5}CrCuFeNi$ | 0.835 | 0.520 | -0.385 | 0.379 | -0.931 | -0.189 | 0.802 | -1.038 | 0.169 | -1.530 | 0.926 | -0.015 | -0.596 | 0.530 | -0.224 |
| CrCuFeNi | - | - | - | - | - | -0.008 | 0.955 | -0.677 | -0.269 | -1.768 | 0.920 | -0.107 | -0.803 | 0.560 | -0.184 |

TABLE S3: Short-range order parameters (first shell) for all element pairs in the final structures of the Monte Carlo MD simulations for the larger boxes (4000 atoms) initially in FCC

| composition | Al-Al | Al-Cr | Al-Cu | Al-Fe | Al-Ni | Cr-Cr | Cr-Cu | Cr-Fe | Cr-Ni | Cu-Cu | Cu-Fe | Cu-Ni | Fe-Fe | Fe-Ni | Ni-Ni |
|---|---|---|---|---|---|---|---|---|---|---|---|---|---|---|---|
| AlCrCuFeNi | 0.430 | 0.303 | -0.251 | 0.030 | -0.513 | -0.564 | 0.622 | -0.609 | 0.241 | -0.808 | 0.629 | -0.186 | -0.475 | 0.440 | 0.028 |
| $AlCrCuFeNi_2$ | 0.555 | 0.504 | -0.318 | 0.293 | -0.517 | -0.572 | 0.786 | -1.075 | 0.178 | -1.120 | 0.750 | -0.049 | -0.706 | 0.370 | 0.009 |
| $AlCrCuFeNi_3$ | 0.699 | 0.632 | -0.427 | 0.473 | -0.459 | -0.528 | 0.835 | -1.170 | 0.077 | -1.235 | 0.780 | 0.016 | -0.844 | 0.254 | 0.037 |
| $Al_{0.5}CrCuFeNi$ | 0.655 | 0.473 | -0.371 | 0.272 | -0.701 | -0.328 | 0.732 | -0.723 | 0.082 | -1.392 | 0.800 | 0.046 | -0.562 | 0.351 | -0.129 |
| CrCuFeNi | - | - | - | - | - | -0.067 | 0.857 | -0.534 | -0.256 | -1.977 | 0.799 | 0.322 | -0.332 | 0.068 | -0.133 |

## S5. FINAL FRAMES AFTER ANNEALING

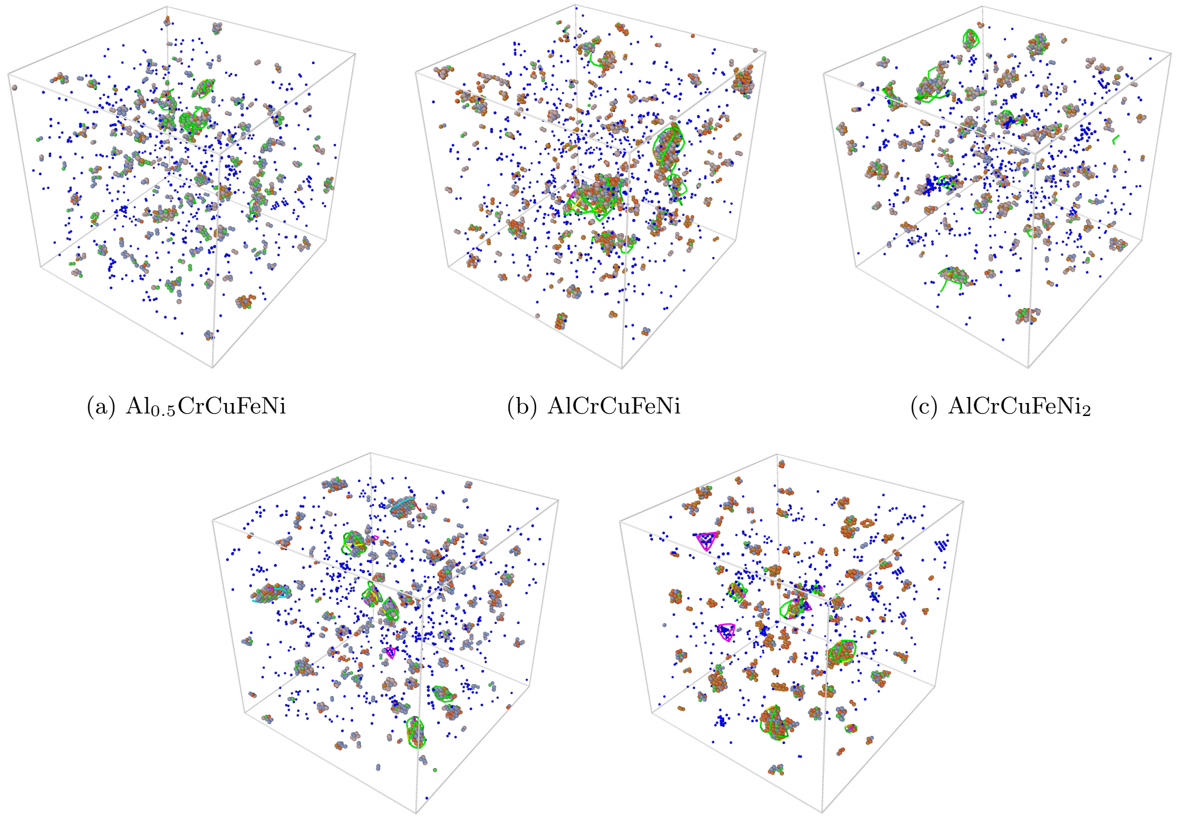

(a) $Al_{0.5}CrCuFeNi$ (b) AlCrCuFeNi (c) $AlCrCuFeNi_2$

(d) $AlCrCuFeNi_3$ (e) CrCuFeNi

FIG. S4: Final configurations after annealing of the 400 consecutive 5 keV collision cascades in the different compositions. Different colored spheres indicate interstitials of different chemical elements and blue spheres indicate vacancies. Additionally, dislocation lines identified from DXA analysis are shown: Green lines represent Shockley dislocations, cyan lines represent Frank dislocations, yellow lines represent Hirth dislocations, Blue lines represent perfect dislocations, pink lines represent stair-rod dislocations and red lines are dislocations of type "other".

## S6. OVERLAPPING CASCADES, WITH NONPHYSICAL MASS OF AL

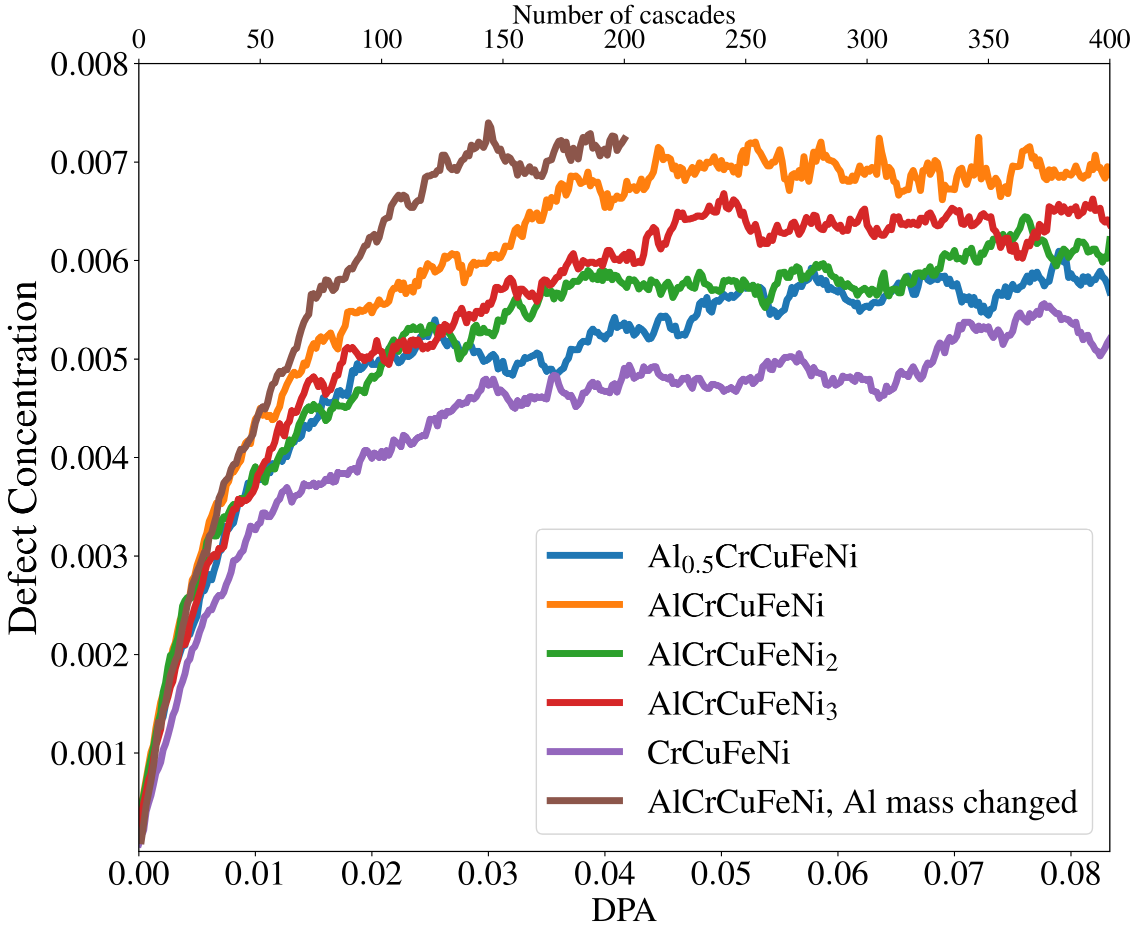


FIG. S5: Defect concentration as a function of estimated dose (NRT dpa) for the different compositions. Here the brown curve indicates the nonphysical simulation where the mass of Al atoms was changed to that of Ni.
